# Supplementary material for: Weighted Connected Matchings
Source: arXiv:2202.04746 source file (2022-02-09)
Supplement: Supplementary file 1 [file appendices.tex]

\newpage
\setcounter{section}{0}

\section*{Appendix}

\section{Proof of Theorem ...}
